# Supplementary material for: TiZero: Mastering Multi-Agent Football with Curriculum Learning and Self-Play
Source: arXiv:2302.07515 source file (2023-02-21)
Supplement: Supplementary file 1 [file Appendix.pdf]

# TiZero Appendix

## A TiZero Visualizations

In this section, we visualize some tactics learned by TiZero. The video of below screen shots can be found at: `https://www.youtube.com/watch?v=U9REh0otmVU`.

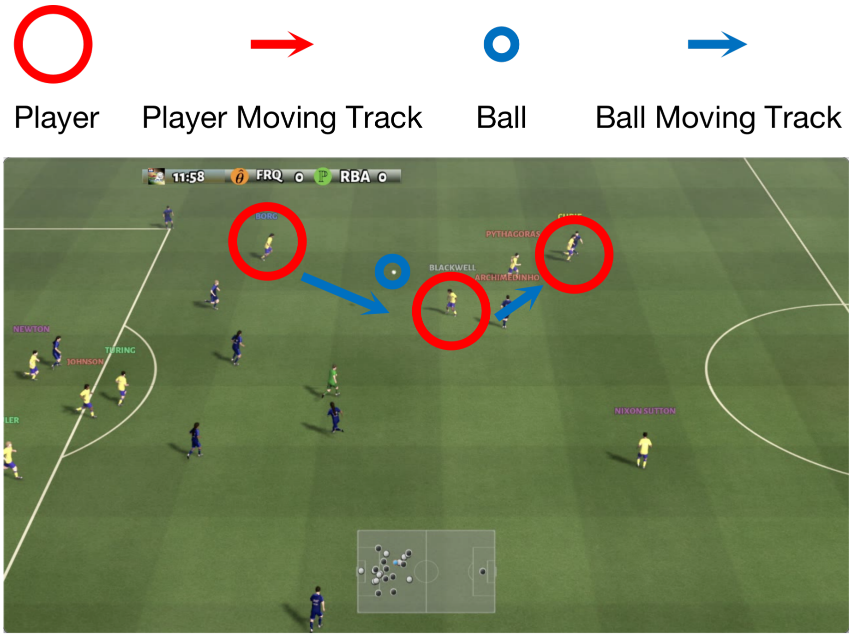


Figure 1: **Quick Counter-attack**. The yellow players under TiZero's control move the ball quickly forward with two successful passes. This sets up the the yellow forward player to outrun the blue defenders and score a goal.

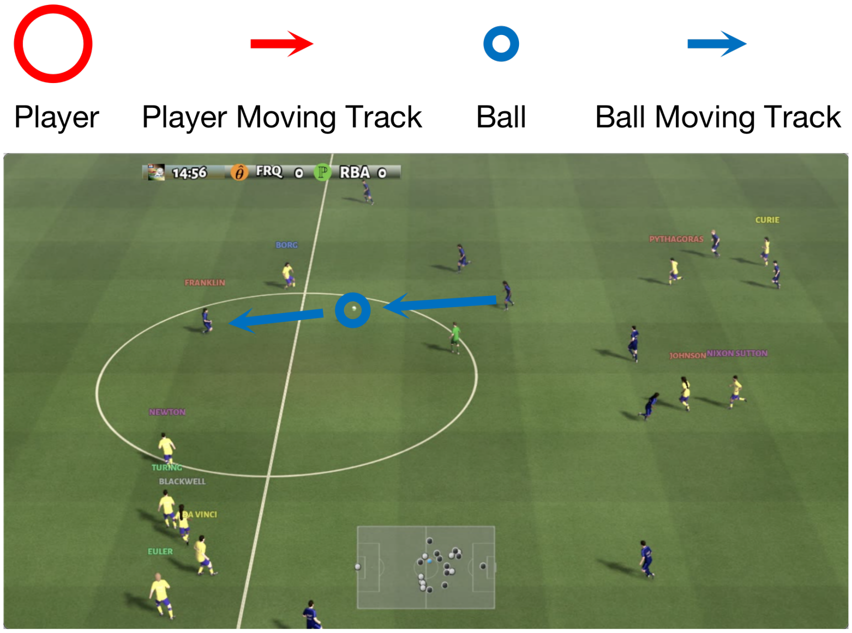


Figure 2: **Offside Trap**. TiZero arranges all defenders in a line high up the pitch. When the opposing blue player passes the ball forward, they are ruled offside, and the yellow team is awarded the ball.

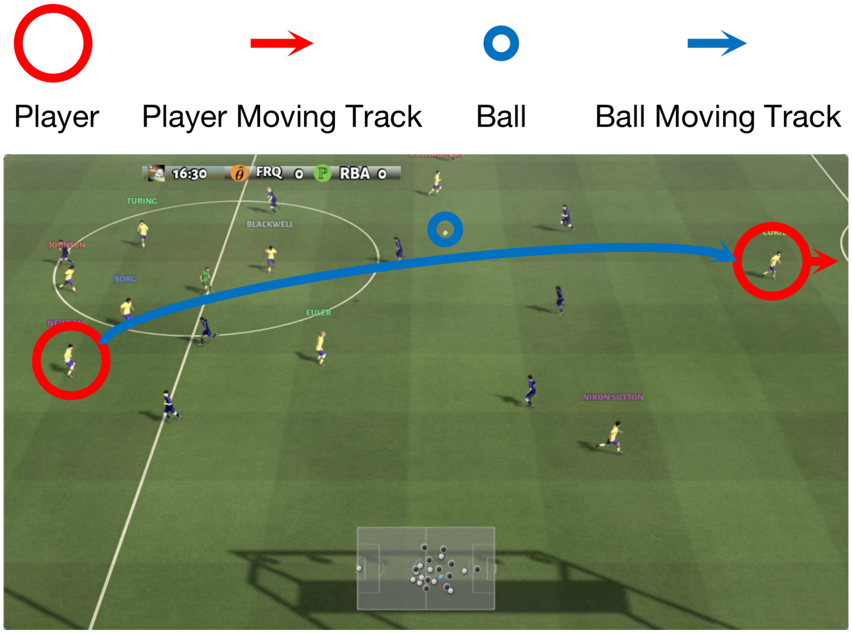


Figure 3: **Attacking Long-Ball**. TiZero utilizes the long-pass action to clear the ball over the opposition's heads for a fast attack. The forward player precisely times their run to avoid being called offside.

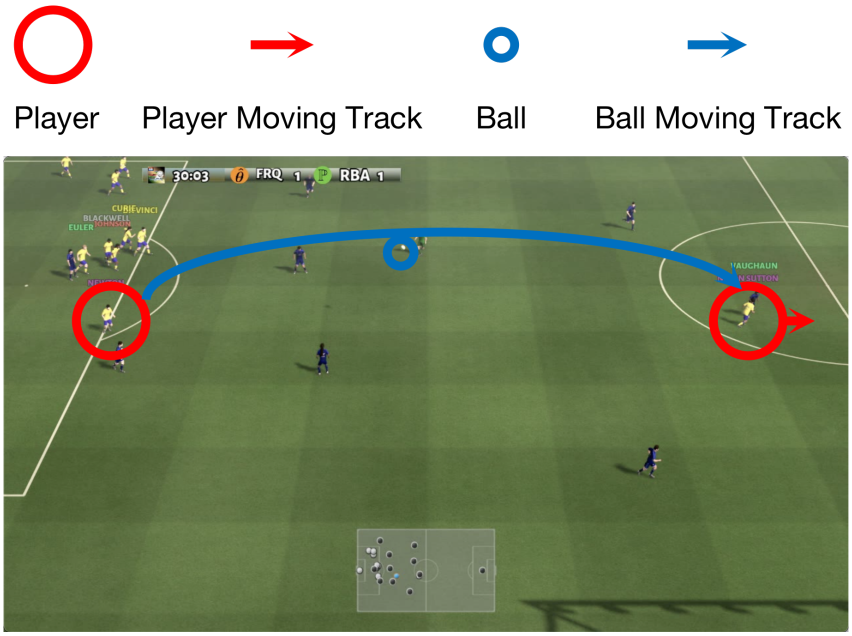


Figure 4: **Defensive Clearance**. TiZero clears the ball when in threatening positions (here under pressure from a blue attack), by making a long-pass up the pitch. Note also that TiZero leaves a single forward player high up the pitch, while committing the majority of the team to defense. This is a common strategy in real-world football.

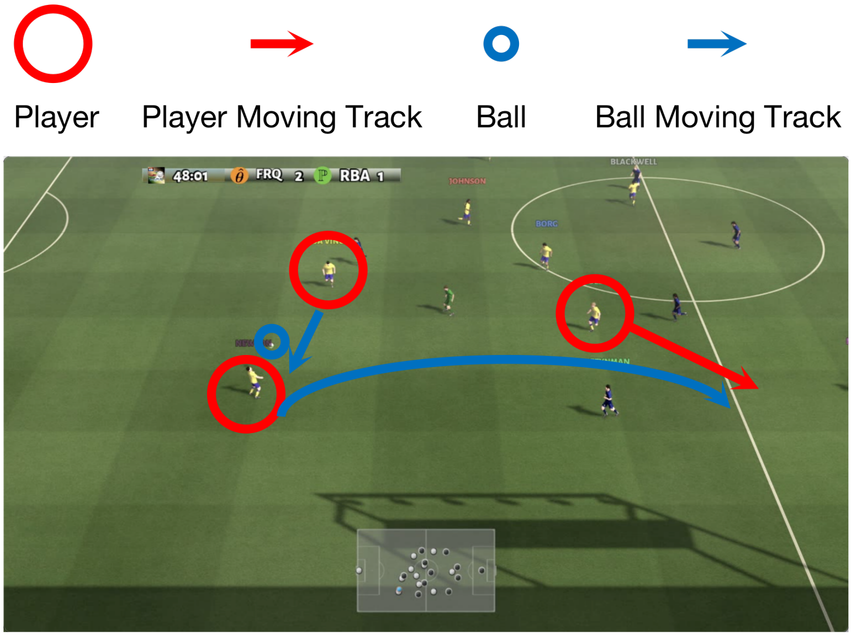


Figure 5: **Pass-and-Move**. TiZero can breakthrough the opponents' midfield and defense through highly coordinated passing and timing of runs.

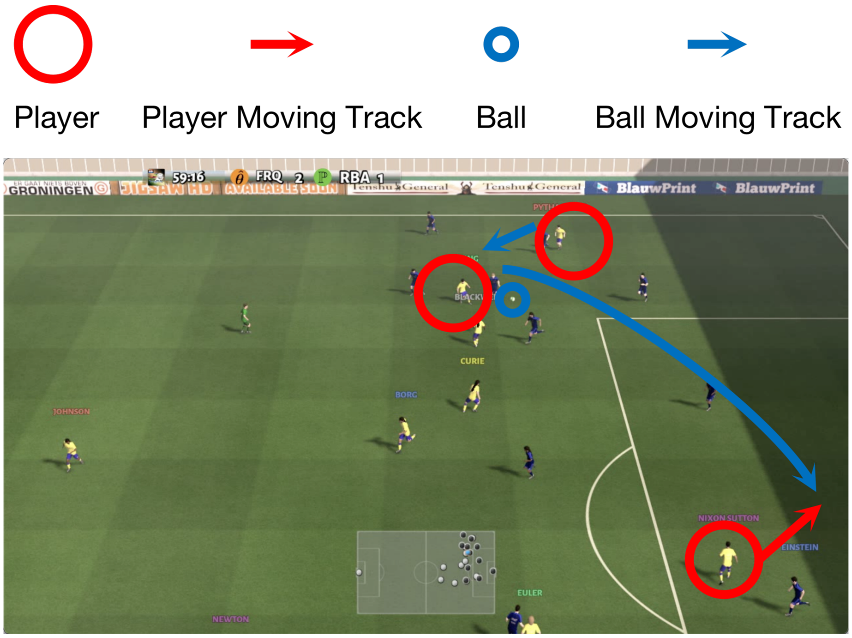


Figure 6: **Crossing from Wings**. TiZero agents take a throw-in followed by a long cross to create a chance for the striker running into the penalty box.

## B Curriculum Design

To relieve the problem of sparse reward when training GFootball agent, we design a curriculum self-play mechanism, in which agents are trained on a sequence of progressively more difficult scenarios, where the opponent is a copy of the agent from the previous difficulty-level scenario. We design ten difficulty levels by configuring the GFootball environment settings. The difficulty level is determined by two aspects; 1) The strength of opponent players, which can be varied from 0 to 1, with values closer to 1 meaning players are quicker and have better stamina. 2) The initial positions of players and the ball. For example, players can be set in positions closer to the opponent's goal. At the beginning of training, agents are initialized with random weights, and learn on the lowest difficulty scenario (lowest opponent strength and positioned closest to the goal). This allows agents to receive denser rewards that encourage basic shooting and passing behaviors. When agent performance meets some threshold in the current scenario, the difficulty level automatically increases. We illustrate the scenarios of different difficulty levels below.

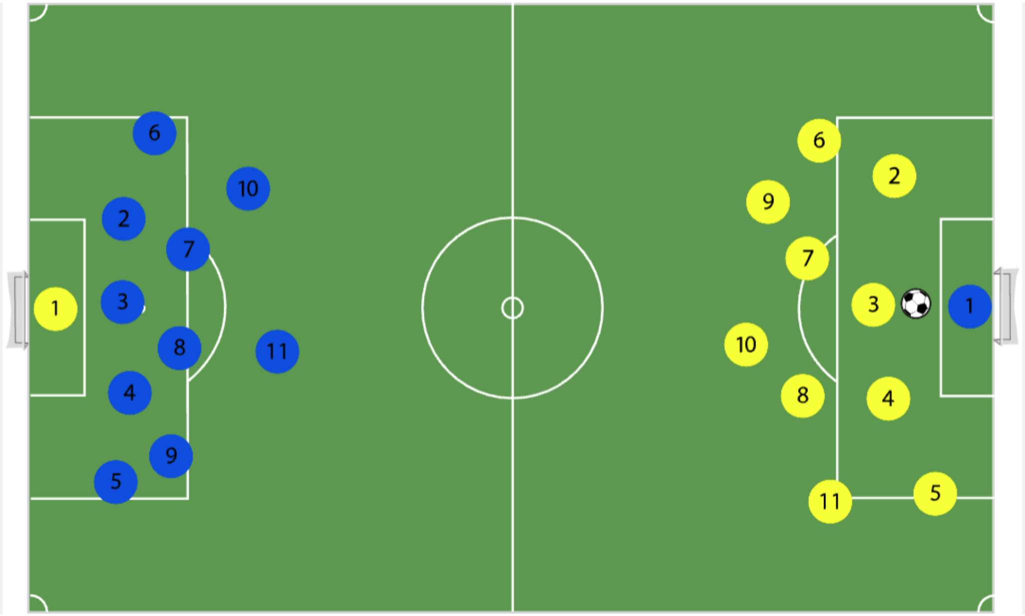


Figure 7: **Difficulty level 1.** This is the initial and easiest difficulty level for the yellow team. The players of the yellow team are set in positions close to the opponent's goal and the ball is also set in position closer to the opponent's goal. It is straightforward for the yellow team to learn how to score a goal.

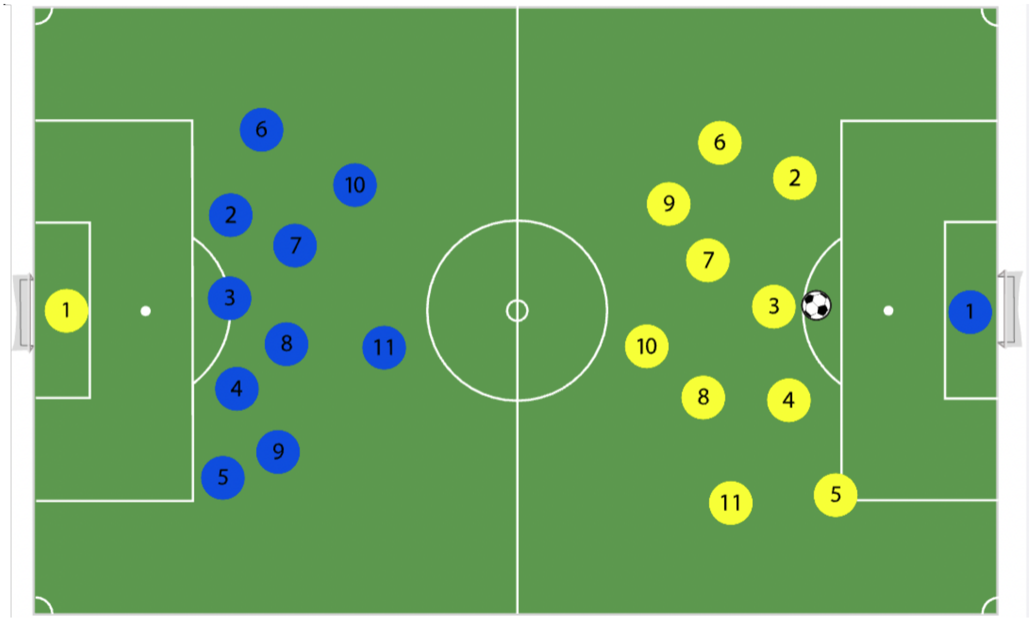


Figure 8: **Difficulty level 5.** When the agents can handle easy situations, the difficulty level is slightly increased. Players of yellow team are set in positions farther from the opponent's goal, along with the ball. In this situation, agents must learn longer-term planning to beat the goal keeper and score a goal.

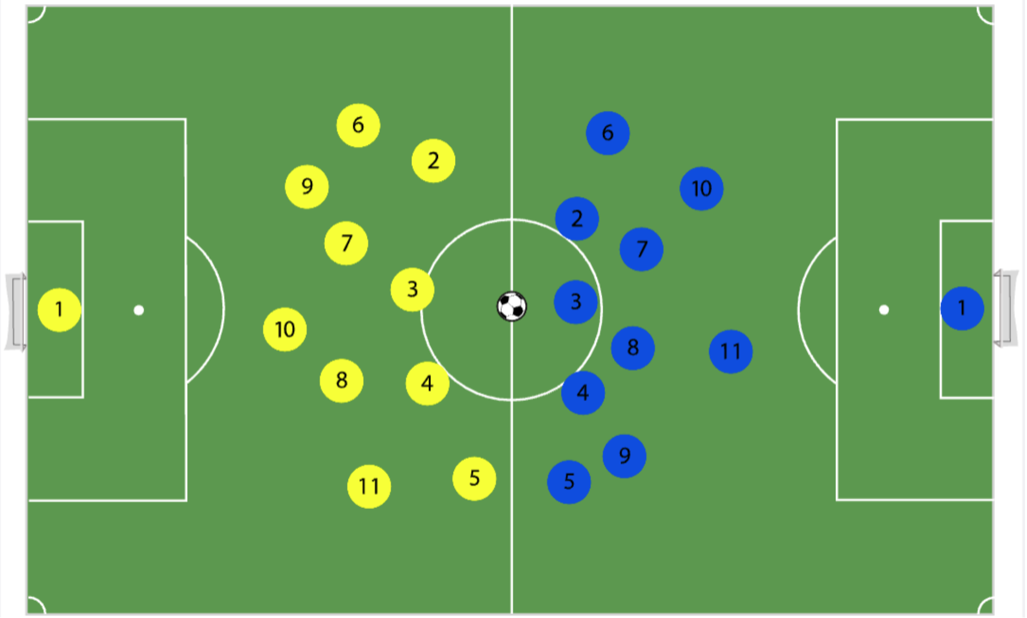


Figure 9: **Difficulty level 10.** This is the most difficult level. Agents must compete with the whole opponent team. This encourages more advanced tactics and team cooperation to score.

## C Challenge & Generalise Self-play

To improve performance against a range of opponents, we design an algorithm that produces a monotonically-improving sequence of policies. This consists of two steps:

1) **Challenge Self-play.** Current agents play against the most recently saved agents with probability of 80%, and play against older versions with probability of 20%. The main purpose of this step is to ensure the current system can defeat the strongest agents seen so far. When the winning rate of current training agent reaches 0.8, the training process will move to next step—the Generalise Self-play.

2) **Generalise Self-play.** Current agents play against the whole opponent pool, sampling opponents according to their strength as follows. Denote the opponent pool $\mathcal{M}$. Let $i \notin \mathcal{M}$ be the current training agent, $j \in \mathcal{M}$ all other agents in pool, and $p(i,j)$ be the probability that agent $i$ defeats agent $j$. We sample model $j$ to play train against with probability:

$$p_{\text{sample}}(j) = \frac{f_{\text{hard}}\left(p(i,j)\right)}{\sum_{m \in \mathcal{M}} f_{\text{hard}}\left(p(i,m)\right)}, \tag{1}$$

where $f_{\text{hard}}(x) = (1-x)^2$. This sampling strategy focuses our agents training on opponents it is less likely to win against. Hence, it maximizes the performance over all existing opponents. Prioritized fictitious self-play addresses the non-transitivity dilemma and improves the robustness of agents [4]. Once agents perform well on this step, they are themselves added to the opponent pool for future versions to train against. In the GFootball, when the average winning rate over the whole opponent pool exceeds 0.8, a new opponent will be saved. The whole process of the our self-play strategy can be found in Algorithm 1

## D Network Architecture of TiZero

For the **policy network**, we use six separate MLPs with two (one for the "player ID") fully-connected layers to separately encode each part of the observation. The hidden size of these MLP layers are set to 64. These extracted hidden features are then concatenated together and processed by an LSTM layer [1], which provides the agent with memory. The hidden size of the LSTM layer is set to 256. All hidden layers have layer normalization and ReLU non-linearities. We use the orthogonal matrix [3] for parameter initialization and the Adam optimizer [2]. To accelerate learning, we mask out any illegal actions by setting their probability of selection to zero. The action output layer is a Softmax layer with a 19-dimension vector. Figure 10 shows the overall policy network architecture:

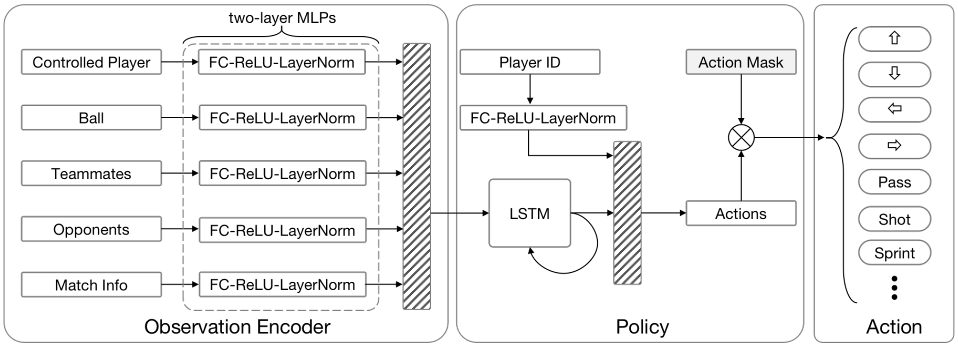


Figure 10: TiZero's policy network architecture. Six types of information are required as input: the controlled player information, player ID, ball information, teammate information, opponent information and current match information. We use six separate MLPs with two (one for the "player ID") fully-connected layers to encode each part of the observation. An LSTM layer is used to incorporate historic observations. The policy outputs a softmax distribution over the 19 discrete actions.

For the **value network**, we use five separate MLPs with two fully-connected layers to separately encode each part of the observation. The hidden size of these MLP layers are set to 64. These

extracted hidden features are then concatenated together and processed by an LSTM layer, which provides the agent with memory. The hidden size of the LSTM layer is set to 256. All hidden layers have layer normalization and ReLU non-linearities. We use the orthogonal matrix for parameter initialization and the Adam optimizer. Figure 11 shows the overall value network architecture:

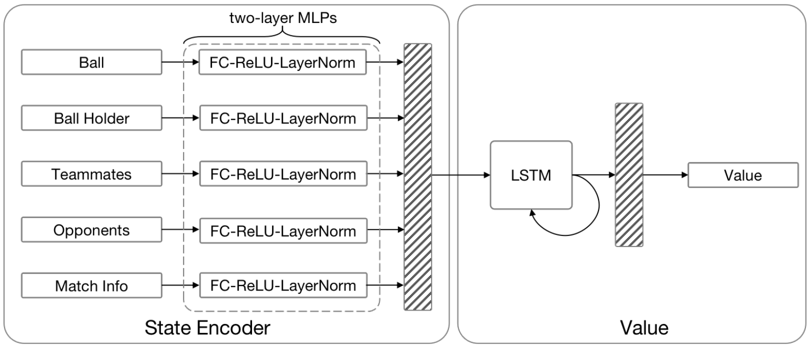


Figure 11: TiZero's value network architecture. Five types of information are required as input: ball information, information of ball holder, teammate information, opponent information and current match information. We use five separate MLPs with two fully-connected layers to encode each part of the observation. An LSTM layer is used to incorporate historic observations. The value network is trained with Mean Square Error (MSE) loss.

# E Public Leaderboard of GFootball Systems

To verify our system independently, we also submitted our best TiZero system to a public evaluation platform[1], which maintains a public leaderboard of GFootball systems. At present, TiZero ranks first with a score of 9.7 and win rate of 95.8%.

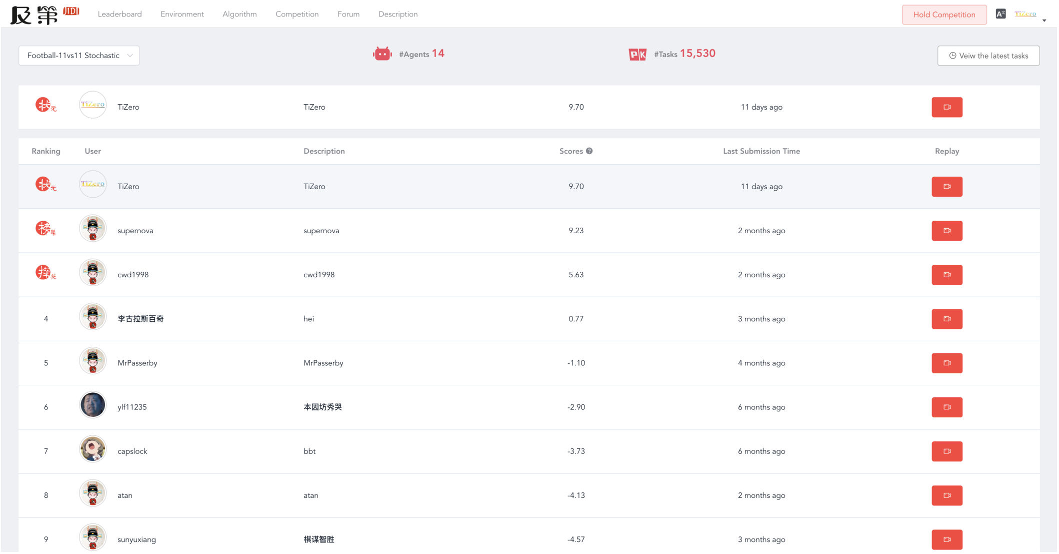


Figure 12: Snapshot of public leaderboard of GFootball systems on JiDi platform.

[1]JiDi AI Competition Platform: `http://www.jidiai.cn/ranking_list?tab=34`. The evaluation result was collected on October 28th, 2022.

## F Self-play Algorithm

**Algorithm 1:** Self-play Strategy

**Initialize:** Randomly initialized policy $\pi_0$, current policy index $i \leftarrow 1$, current policy $\pi_i \leftarrow \pi_0$, opponent pool $\mathcal{M} := \{\pi_0\}$.
**Let:** $p_{\text{win}}(\pi_i, \mathcal{P})$ be the winning rate of policy $\pi_i$ against an opponent set $\mathcal{P}$.
**Stage 1: Curriculum Self-play:**
    **Initialize:** current difficulty level $L_{\text{diff}} \leftarrow 0$, maximal difficulty level $L_{\text{max}}$, winning rate threshold $\eta_{\text{stage\_1}}$.
    **Initialize:** set environment difficulty to $L_{\text{diff}}$.
    **while** $L_{\textit{diff}} < L_{\textit{max}}$ **do**
        $\pi_i \leftarrow \text{JRPO\_Training}(\pi_i, \pi_{i-1})$
        **if** $p_{\textit{win}}(\pi_i, \{\pi_{i-1}\}) > \eta_{\textit{stage\_1}}$ **then**
            $\mathcal{M} \leftarrow \mathcal{M} \cup \{\pi_i\}$
            $i \leftarrow i + 1$
            $L_{\text{diff}} \leftarrow L_{\text{diff}} + 1$
            Set environment difficulty to $L_{\text{diff}}$.
        **end**
    **end**
**End Stage 1**
**Stage 2: Challenge & Generalise Self-play:**
    **Initialize:** winning rate threshold $\eta_{\text{step\_1}}$ and $\eta_{\text{step\_2}}$.
    **while** *Not Converged* **do**
        **Step 1: Challenge Self-play:**
            **for** *each episode* **do**
                Set opponent as most recent agent, $\pi_j = \pi_{i-1}$, with 80% probability. Else sample $\pi_j \sim \{\pi_k\}_{k<(i-1)}$ uniformly.
                $\pi_i \leftarrow \text{JRPO\_Training}(\pi_i, \pi_j)$
                **if** $p_{\textit{win}}(\pi_i, \{\pi_{i-1}\}) > \eta_{\textit{step\_1}}$ **then**
                    **Break**
                **end**
            **end**
        **End Step 1**
        **Step 2: Generalise Self-play:**
            **for** *each episode* **do**
                Sample opponent policy $\pi_j$ from opponent pool $\mathcal{M}$ based on win rates, eq. 1.
                $\pi_i \leftarrow \text{JRPO\_Training}(\pi_i, \pi_j)$
                **if** $p_{\textit{win}}(\pi_i, \mathcal{M}) > \eta_{\textit{step\_2}}$ **then**
                    $\mathcal{M} \leftarrow \mathcal{M} \cup \{\pi_i\}$
                    $i \leftarrow i + 1$
                    **Break**
                **end**
            **end**
        **End Step 2**
    **end**
**End Stage 2**

## G Environments

In this section, we will introduce each environment used in our experiments.

### G.1 Overcooked

Overcooked is a grid kitchen game in which agents cooperate to complete a series of tasks, such as finding vegetables, making soup and delivering food.

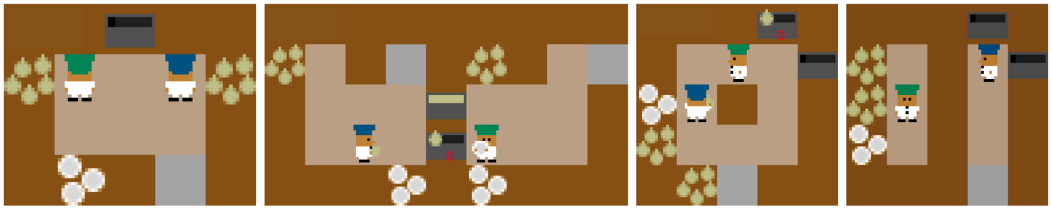

Figure 13: **Screen shots of Overcooked**. From left to right: *simple*, *unident*, *random1*, *random0*.

### G.2 MPE

MPE is a 2D world with multiple movable particles. Agents have to learn to cover all the landmarks while avoiding collisions. Agents are rewarded based on how far any agent is from each landmark. Agents are penalized if they collide with other agents.

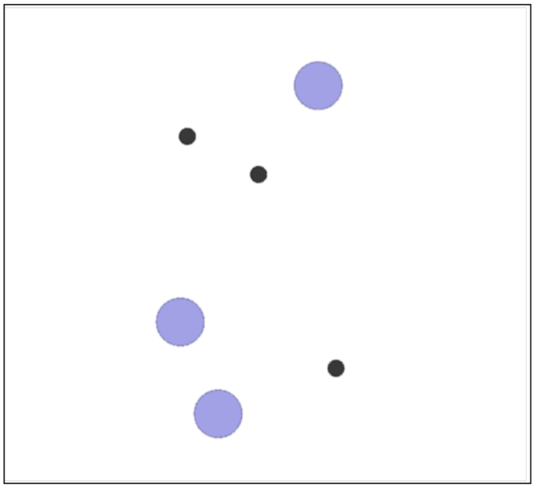

Figure 14: **Screen shots of MPE**. The blue particles are movable particles controlled by agents, and the black particles are the target landmarks which need to be covered by blue particles.

### G.3 Tic-Tac-Toe

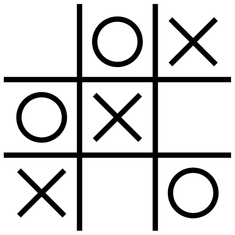

Figure 15: **Screen shots of Tic-Tac-Toe**. There are three 'X's on the diagonal, thus the player who plays the 'X' win the game.

In the Tic-Tac-Toe game, two players take turns placing marks on a three-by-three grid. Players win by placing three of their marks in a line. Our agent is a deep neural network with a 27-dimension state vector as input (O's, X's and blanks are one-hot encoded for the 9 cells)

### G.4 Connect-Four

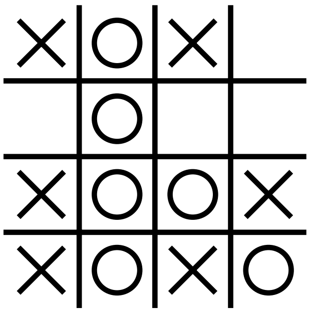

Figure 16: **Screen shots of Connect-Four**. There are four 'O's on the second column, thus the player who plays the 'O' win the game.

In the Connect-Four game, two players take turns placing marks on a four-by-four grid. Players win by placing four of their marks in a line. Our agent is a deep neural network with a 48-dimension state vector as input (O's, X's and blanks are one-hot encoded for the 16 cells)

## H Hyperparamters of GFootball and TiZero

We train and evaluate TiZero on the full 11 vs. 11 game mode in GFootball. Each match lasts for five minutes, or $3,000$ timesteps (no extra time). The team with highest number of goals wins. Standard football rules are applied by the game, such as offside, penalty kicks and yellow/red cards. TiZero was trained over 45 days on a cluster with 800 CPUs and two NVIDIA A100 GPUs. The batch size for each GPU is set to $2,150,000$, the hidden size of the LSTM layer is 256, and the discount factor $\gamma$ is $0.999$. We used the Adam optimizer with learning rate of $0.0001$. More hyper-parameters are summarized as bellow:

| Hyper-Parameters | Value |
|---|---|
| recurrent data chunk length | 25 |
| episode length | 500 |
| game length | 3000 |
| max clipped value loss | 0.2 |
| gradient clip norm | 10.0 |
| GAE $\lambda$ | 0.995 |
| discount factor $\gamma$ | 0.999 |
| value loss | huber loss |
| huber $\delta$ | 10.0 |
| number of LSTM layers | 1 |
| RNN hidden state dim | 256 |
| fc layer dim | 64 |
| learning rate | 1e-4 |
| gain | 0.01 |
| number of parallels for each actor rollout | 10 |
| entropy coefficient | 0.01 |
| ppo update number | 2 |
| pass ball reward | 0.05 |
| gather penalty | 0.001 |
| out of boundary penalty | 0.001 |
| hold ball reward | 1e-4 |

Table 1: Hyper-parameters used in TiZero.

# I Hyperparameters of Multi-agent Reinforcement Learning

In this section, we list the hyperparameters used in Overcooked and MPE. To evaluate MARL algorithms, we used a platform involves a 256-core CPU, 2TB RAM, and an NVIDIA A100 with 80GB VRAM.

| Hyper-Parameters | Value |
|---|---|
| recurrent data chunk length | 10 |
| episode length | 400 |
| max clipped value loss | 0.2 |
| gradient clip norm | 10.0 |
| GAE $\lambda$ | 0.95 |
| discount factor $\gamma$ | 0.99 |
| value loss | huber loss |
| huber $\delta$ | 10.0 |
| number of GRU layers | 1 |
| RNN hidden state dim | 64 |
| fc layer dim | 64 |
| learning rate | 7e-4 |
| gain | 0.01 |
| number of parallels for each actor rollout | 128 |
| entropy coefficient | 0.01 |
| ppo update number | 10 |

Table 2: Hyper-parameters used in Overcooked.

| Hyper-Parameters | Value |
|---|---|
| recurrent data chunk length | 10 |
| episode length | 25 |
| max clipped value loss | 0.2 |
| gradient clip norm | 10.0 |
| GAE $\lambda$ | 0.95 |
| discount factor $\gamma$ | 0.99 |
| value loss | huber loss |
| huber $\delta$ | 10.0 |
| number of GRU layers | 1 |
| RNN hidden state dim | 64 |
| fc layer dim | 64 |
| learning rate | 7e-4 |
| gain | 0.01 |
| number of parallels for each actor rollout | 100 |
| entropy coefficient | 0.01 |
| ppo update number | 10 |

Table 3: Hyper-parameters used in MPE.

## J Hyperparameters of Self-play Strategies

In this section, we list the hyperparameters used in Tic-Tac-Toe and Connect-Four. To evaluate self-play strategies, we used a platform involves a 256-core CPU, 2TB RAM, and an NVIDIA A100 with 80GB VRAM.

| Hyper-Parameters | Value |
|---|---|
| recurrent data chunk length | 1 |
| episode length | 20 |
| max clipped value loss | 0.2 |
| gradient clip norm | 10.0 |
| GAE $\lambda$ | 0.995 |
| discount factor $\gamma$ | 0.999 |
| value loss | huber loss |
| huber $\delta$ | 10.0 |
| number of GRU layers | 1 |
| RNN hidden state dim | 32 |
| fc layer dim | 32 |
| learning rate | 7e-4 |
| gain | 0.01 |
| number of parallels for each actor rollout | 200 |
| entropy coefficient | 0.05 |
| ppo update number | 5 |

Table 4: Hyper-parameters used in Tic-Tac-Toe.

| Hyper-Parameters | Value |
|---|---|
| recurrent data chunk length | 1 |
| episode length | 20 |
| max clipped value loss | 0.2 |
| gradient clip norm | 10.0 |
| GAE $\lambda$ | 0.995 |
| discount factor $\gamma$ | 0.999 |
| value loss | huber loss |
| huber $\delta$ | 10.0 |
| number of GRU layers | 1 |
| RNN hidden state dim | 32 |
| fc layer dim | 32 |
| learning rate | 7e-4 |
| gain | 0.01 |
| number of parallels for each actor rollout | 200 |
| entropy coefficient | 0.05 |
| ppo update number | 5 |

Table 5: Hyper-parameters used in Connect-Four.

# K Experiments on Multi-agent Reinforcement Learning

In this section, we add more experimental results of multi-agent algorithms on Overcooked and MPE.

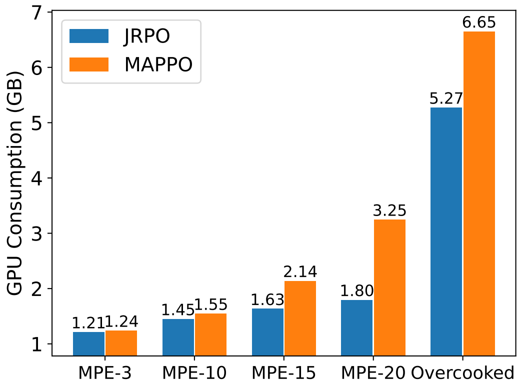


(a)

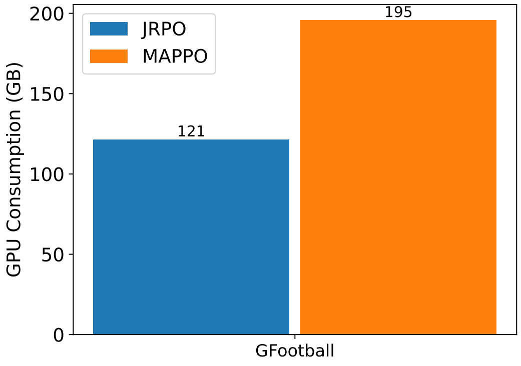


(b)

Figure 17: (a) & (b) GPU memory consumption of different methods. The lower the better. Results show that JRPO consumes less GPU memory than MAPPO.

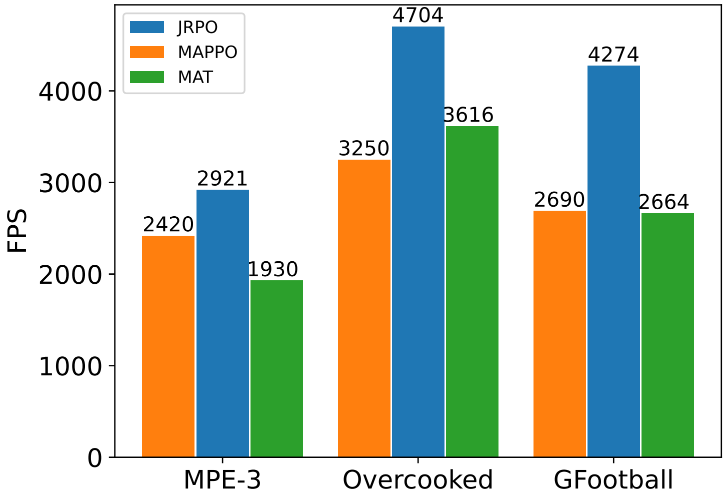


Figure 18: Training speed (frames per second, FPS) of different methods. Results show that JRPO trains 1.2× quicker on MPE, 1.4× quicker on Overcooked, 1.6× quicker on GFootball.

## L Self-play Experiments

We visualize state embeddings of policies produced by different self-play strategies in Figure 19, and points are colored according to different strategies.

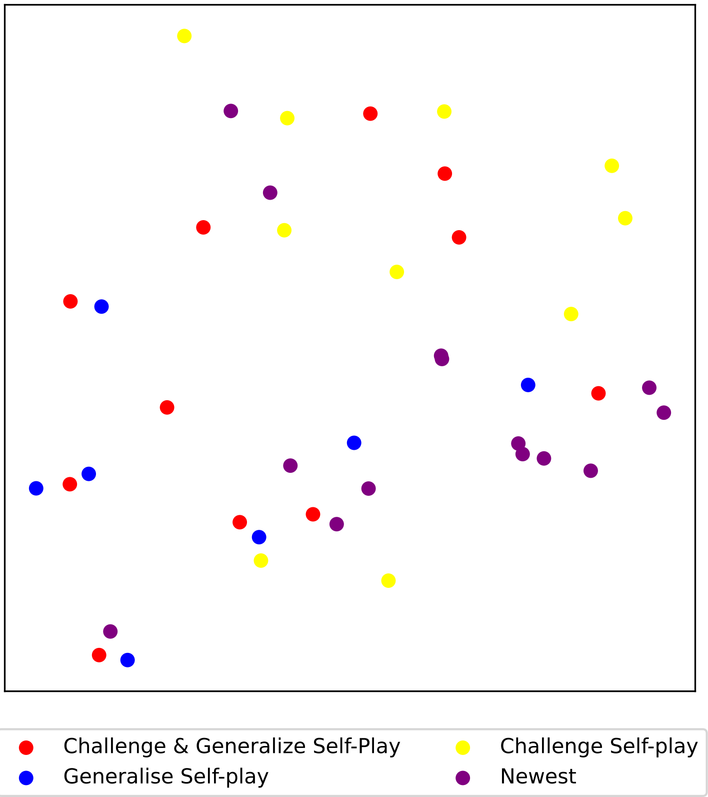


Figure 19: State t-SNE embeddings of policies produced by different self-play strategies.

## M Observation Design

In this section , we will describe the detailed observation design for TiZero. We split the agent observation into six parts, including the controlled player information, player ID, ball information, teammate information, opponent information and current match information. We also design a global state vector for the value-network with five parts, including ball information, information of ball holder, teammate information, opponent information and current match information.

Table 6: Controlled player information: 87 dimensions.

| |
|---|
| sticky actions |
| current position |
| current direction |
| tired factor |
| yellow card |
| red card |
| offside |
| relative ball position |
| distance to ball |
| relative teammate positions |
| distance to teammates |
| relative opponent positions |
| distance to opponents |

Table 7: Player ID: 11 dimensions.

| |
|---|
| player ID |

Table 8: Ball information: 57 dimensions.

| |
|---|
| ball position |
| ball direction |
| ball owned team |
| ball rotation |
| ball owned player |
| current player information |
| ball owned player position |
| ball owned player direction |
| relative position of ball owner |
| distance to ball owner |
| ball owner information |

Table 9: Teammate information: 88 dimensions (this is also for value network).

| |
|---|
| teammate positions |
| teammate directions |
| teammate tired factors |
| teammate yellow cards |
| teammate red cards |
| teammate offside |

Table 10: Opponent information: 88 dimensions (this is also for value network).

| |
|---|
| opponent positions |
| opponent directions |
| opponent tired factors |
| opponent yellow cards |
| opponent red cards |
| opponent offside |

Table 11: Current match information: 9 dimensions (this is also for value network).

| |
|---|
| game mode |
| goal differences |
| remaining steps |

Table 12: Ball information for value network: 12 dimensions.

| |
|---|
| ball position |
| ball direction |
| ball rotation |
| ball owned team |

Table 13: Ball owned player information for value network: 23 dimensions.

| |
|---|
| ball owned player ID |

# References

[1] Sepp Hochreiter and Jürgen Schmidhuber. Long short-term memory. *Neural computation*, 9(8):1735–1780, 1997.

[2] Diederik P Kingma and Jimmy Ba. Adam: A method for stochastic optimization. *arXiv preprint arXiv:1412.6980*, 2014.

[3] Andrew M Saxe, James L McClelland, and Surya Ganguli. Exact solutions to the nonlinear dynamics of learning in deep linear neural networks. *arXiv preprint arXiv:1312.6120*, 2013.

[4] Oriol Vinyals, Igor Babuschkin, Wojciech M Czarnecki, Michaël Mathieu, Andrew Dudzik, Junyoung Chung, David H Choi, Richard Powell, Timo Ewalds, Petko Georgiev, et al. Grandmaster level in starcraft ii using multi-agent reinforcement learning. *Nature*, 575(7782):350–354, 2019.
